# Supplementary material for: Light Clients for Lazy Blockchains
Source: arXiv:2203.15968 source file (2024-05-04)
Supplement: Supplementary file 1 [file appendix_execution_oracles.tex]

We first observe that the UTXO model can also be captured by the construction given in Section~\ref{sec:execution-oracle}, where in this case, state elements at the leaves of the SMT would be the UTXOs.
However, we also give an alternative construction that could be of independent interest.
For this purpose, we first focus on a hypothetical data structure for which the following assumptions hold:
\begin{enumerate}
\item Given any two transactions $\tx$ and $\tx'$, one can check if there is a conflict or dependency arrow from $\tx'$ to $\tx$ in time that is polynomial in the size of the transactions.
\item A transaction $\tx$ is valid if both of the following conditions hold:
  \begin{enumerate}
  \item All transactions $\tx' \preceq \tx$ such that there is a conflict arrow from $\tx'$ to $\tx$ are invalid.
  \item All transactions $\tx' \preceq \tx$ such that there is a dependency arrow from $\tx'$ to $\tx$ are valid.
  \end{enumerate}
\end{enumerate}
We observe that the UTXO model satisfies these assumptions, thus can use this following data structures for the \eoracle.

A full node keeps two separate directed graphs in its memory called the \emph{conflict graph} and \emph{dependency graph} respectively.
At any given time $t$, both graphs contain as vertices all of the transactions the full node $v$ has seen on the dirty ledger $\LOGdirty{v}{t}$ of its view by that time.
Conflict and dependency graphs represent the conflict and dependency arrows between these transactions as edges.
In this context, there exists a directed edge from a transaction $\tx_1$ to $\tx_2$ in the conflict graph if
(i) $\tx_1 \preceq \tx_2$ in the dirty ledger, and (ii) there exists a conflict arrow from $\tx_1$ to $\tx_2$.
Note that (i) and (ii) together implies that if $\tx_1$ is valid, then $\tx_2$ has to be invalid.
Similarly, there exists a directed edge from a transaction $\tx_1$ to $\tx_2$ in the dependency graph if
(i) $\tx_1 \preceq \tx_2$ in the dirty ledger, and (ii) there exists a dependency arrow from $\tx_1$ to $\tx_2$.
Thus, (i) and (ii) together implies that if $\tx_1$ is invalid, then $\tx_2$ has to be invalid as well.
We stipulate that these graphs are stored in the form of Merkle trees.

Finally, suppose a light client queries this \eoracle at phase 2 of the bisection game described in Section~\ref{sec:bisection-game}.
Moreover, assume that the full nodes simply record the validity information and the Merkle roots for dependency and conflict arrows as their state roots at each leaf of their dirty trees.
Then, a full node can prove to the light client succinctly that the transaction included at the disputed leaf is invalid by showing either a conflict arrow from a previous valid transaction or a dependency arrow from a previous invalid transaction, along with the Merkle inclusion proofs for these arrows.
These proofs along with the arrows themselves correspond to the auxiliary data $\aux$ in our formulation in Section~\ref{sec:execution-oracle}.
Thus, if the light client does not hear a proof of invalidity for a transaction upon querying the \eoracle, it knows that the transaction is valid, as long as there is an honest full node in the audience.

Succinctness, completeness and soundness of the \eoracle constructions will be provided in a future iteration of this work.
