# Supplementary material for: Light Clients for Lazy Blockchains
Source: arXiv:2203.15968 source file (2024-05-04)
Supplement: Supplementary file 2 [file appendix_utxo_bisection_game.tex]

\section{SPV Protocol for the UTXO Model}\label{sec:SPV-protocol-for-the-UTXO-model}

When queried by a light client (verifier) for a transaction $\tx$ that is in the dirty ledger of its view, a full node (prover) first shows a Merkle proof of $\tx$'s inclusion within some confirmed block $b$.
It then responds with $\tx$'s color and the roots and sizes of the MMR for the leaves ending at $\tx$.

Upon hearing multiple responses from full nodes, the light client first selects two full nodes that have responded with different colors and thus, different MMR roots.
It then mediates a challenge between these two full nodes, as a result of which client can generate a proof that the MMR roots calculated by one of the nodes is incorrect.
(Note that this does not mean the other party's MMR roots are necessarily correct.)
Thus, it eliminates the node with the incorrect root and continues this process until all of the remaining responses attest to the same color for $\tx$.
It then outputs this color.

We next describe the challenge between two full nodes, during which one node is designated as the challenger and the other one as the responder.
Challenger communicates with the responded through the light client which observes all of the messages.
Challenge is run simultaneously in both directions between the two nodes and described for one direction below.

First, challenger identifies the earliest MMR root that is different from its roots.
It then checks if the size of the Merkle tree corresponding to that root is different from the size of its tree.
If the sizes are different, challenger takes the minimum of the two sizes and identifies the subtree of the larger Merkle tree that corresponds to the smaller one.
Then, it runs the following process starting at the root of the subtree:

Challenger asks the verifier to reveal the two children under the given node along with the proof that they are committed by the root of the whole Merkle tree.
Challenger selects the left child among the hashes revealed by the responder if it is different from the corresponding left child within its Merkle tree, otherwise it selects the right child.
It continues this process of asking the responder to reveal hashes until both parties reach a leaf with index $\idx$.
Let $\leaf_c$ and $\leaf_r$ denote the challenger's and responder's sequences of leaves respectively.

Next, challenger checks if $\leaf_c[\idx].\tx$ is the same as $\leaf_v[\idx].\tx$.
If not, it proves to the client that $\leaf_c[\idx].\tx$ is the transaction that directly follows $\leaf_c[\idx-1].\tx$ on the dirty ledger by showing Merkle inclusion proofs to the appropriate block headers on the ledger.
In this case, challenger succeeds and the client eliminates the responder from its list of nodes.

Second, challenger checks if $\leaf_c[\idx].\mroot$ is the same as $\leaf_v[\idx].\mroot$.
