# Supplementary material for: Light Clients for Lazy Blockchains
Source: arXiv:2203.15968 source file (2024-05-04)
Supplement: Supplementary file 3 [file appendix_utxo_dirty_tree.tex]

\section{Data Structures for the UTXO Model}\label{sec:data-structures-for-the-UTXO-model}

We first focus on the data structures used by the SPV protocol of the execution engines for which the following assumptions hold:
\begin{enumerate}
\item Given any two transactions $\tx$ and $\tx'$, one can check if there is a conflict or dependency arrow from $\tx'$ to $\tx$ in time that is polynomial in the size of the transactions.
\item A transaction $\tx$ is valid if both of the following conditions hold:
  \begin{enumerate}
  \item All transactions $\tx' \preceq \tx$ such that there is a conflict arrow from $\tx'$ to $\tx$ are invalid.
  \item All transactions $\tx' \preceq \tx$ such that there is a dependency arrow from $\tx'$ to $\tx$ are valid.
  \end{enumerate}
\end{enumerate}
We observe that the UTXO model satisfies these assumptions, thus can use the following data structures for SPV.

A full node keeps two separate directed graphs in its memory called the \emph{conflict graph} and \emph{dependency graph} respectively.
At any given time $t$, both graphs contain as vertices all of the transactions the full node $v$ has seen on the dirty ledger $\LOGdirty{v}{t}$ of its view by that time.
Conflict and dependency graphs represent the conflict and dependency arrows between these transactions as edges.
In this context, there exists a directed edge from a transaction $\tx_1$ to $\tx_2$ in the conflict graph if
(i) $\tx_1 \preceq \tx_2$ in the dirty ledger, and (ii) there exists a conflict arrow from $\tx_1$ to $\tx_2$.
Note that (i) and (ii) together implies that if $\tx_1$ is valid, then $\tx_2$ has to be invalid.
Similarly, there exists a directed edge from a transaction $\tx_1$ to $\tx_2$ in the dependency graph if
(i) $\tx_1 \preceq \tx_2$ in the dirty ledger, and (ii) there exists a dependency arrow from $\tx_1$ to $\tx_2$.
Thus, (i) and (ii) together implies that if $\tx_1$ is invalid, then $\tx_2$ has to be invalid as well.
Observe that the full nodes can use a single graph with a single set of vertices and two kinds of edges (conflict and dependency) for memory and computational efficiency.
However, for the ease of explanation, we will keep the two graphs separate in the explanations below.

Validity of transactions are expressed with colors on the dependency and conflict graphs.
A vertex is colored green (red) if the corresponding transaction is valid (invalid).
We observe that a green vertex cannot have an edge coming from another green vertex on the conflict graph.
Similarly, we observe that a green vertex cannot have an edge coming from a red vertex on the dependency graph.

Full nodes commit to the conflict and dependency graphs using Merkle mountain ranges (MMRs).
Given some node $v$'s view at time $t$, leaves of the MMRs are data structures corresponding to transactions on the dirty ledger $\LOGdirty{v}{t}$ augmented by the validity and edge information.
Focusing on the view of a single node at a given time, we omit the identifiers $v$ and $t$ in the description below.
Let $\leaf{v}{t}[i]$ denote the $i$-th leaf in the MMR.
Similarly, let $\edge{v}{t}[i]$ denote the Merkle tree with root $\edge[i].\mroot$ which has as leaves the sequence of indices $j \leq i$ such that there is an edge from the transaction $\LOGdirty[j]$ to $\LOGdirty[i]$ on the conflict graph.
Then, $\leaf[i]$ consists of the following three components: the transaction $\leaf[i].\tx = \LOGdirty[i]$ at height $i$ of the dirty ledger,
the Merkle root $\leaf[i].\mroot=\edge[i].\mroot$ of the sequence of edges ending at that transaction, and the color $\leaf[i].\vcolor$ of the transaction (a single bit).

Upon observing a new transaction $\tx$ in its dirty ledger, a full node first updates the conflict and dependency graph of its transactions.
For this purpose, the node identifies all transactions in the prefix of $\tx$ with a conflict or dependency arrow to $\tx$
and adds an edge between $\tx$ and those transactions.
It then adds a new leaf $\leaf[h(\tx)]$ to the MMR for the new transaction, complete with its color and edge information.
Note that this operation does not require changing any of the existing leaves and takes time polynomial in the total size of the ledger.
