# Supplementary material for: Light Clients for Lazy Blockchains
Source: arXiv:2203.15968 source file (2024-05-04)
Supplement: Supplementary file 4 [file appendix_duplicates.tex]

In this section, we relax the uniqueness assumption for the transactions in the dirty ledgers on lazy blockchain protocols.
Towards this goal, we \emph{deduplicate} transactions by labelling them with unique identifiers from the underlying lazy protocol.

Consider a lazy blockchain protocol which outputs a header chain of blocks each containing the Merkle tree root of the transactions organized within it.
We augment each dirty ledger entry, which contains a transaction $\tx$ and a state commitment $\stc$, by adding the index of the header of the block $B_{\tx}$ containing $\tx$, and the index of the transaction $\tx$ within the Merkle tree of block $B_{\tx}$.
In this case, the verifiers query the \coracle not only with transactions $\tx$ and $\tx' \neq \tx$, but also with their block header indices $j_{\tx}$ and $j_{\tx'}$ and Merkle tree indices $i_{\tx}$ and $i_{\tx'}$.
For the queries, the verifier downloads all the block headers and determines the longest stable header chain.
Then, it asks a prover if $\tx$ immediately precedes $\tx'$ on its dirty ledger.

To affirm, the prover replies with:
\begin{itemize}
    \item the positions $i$ and $i'$ of the transactions $\tx$ and $\tx'$ within their respective Merkle trees,
    \item the Merkle proofs $\pi$ and $\pi'$ from the transactions $\tx$ and $\tx'$ to the corresponding transaction roots,
    \item the positions $j \leq j'$ of the block headers containing these transaction roots, on the longest stable header chain.
\end{itemize}
Then, the verifier checks that the Merkle proofs are valid, $j=j_{\tx}$, $j'=j_{\tx'}$, $i=i_{\tx}$, $i'=i_{\tx'}$, and accepts the prover's claim if and only if either of the following cases hold:
\begin{enumerate}
\item $B_{\tx}$ and $B_{\tx'}$ are the same block, \ie, $j_{\tx'}=j_{\tx}$, and $i=i_{\tx'}=i_{\tx}+1$.
\item $B_{\tx}$ and $B_{\tx'}$ are consecutive, \ie, $j_{\tx'}=j_{\tx}+1$, and $i_{\tx}$ is the index of the last leaf in the tree of block $B_{\tx}$ while $i_{\tx'}$ is the first leaf in the tree of block $B_{\tx'}$.
\end{enumerate}
If no prover is able to provide such a proof, the oracle returns \emph{false} to the verifier.
